# Supplementary material for: House-GAN: Relational Generative Adversarial Networks for Graph-constrained House Layout Generation
Source: arXiv:2003.06988 source file (2020-03-16)
Supplement: Supplementary file 1 [file 9_additional_results.tex]

\section{Additional results}
Figures \ref{fig:results_1}-\ref{fig:results_10} present additional generation results by the proposed system (House-GAN). Each row shows an input bubble diagram and pairs of a generated room mask and the corresponding house layout.
%generated room masks and their corresponding house layout by the proposed approach (House-GAN).
We divide the samples into 5 groups depending on the numbers of rooms. We present two pages of results for each group, in a increasing order of the room counts.
%instance of House-GAN trained and tested on graphs of different sizes.

% xxxxxxxx MENTION that now different figures show graphs with different sizes... xxxxx
%instance trained and tested on graphs of size 1-12 and 13+, respectively. 

\begin{figure*}[t]
\centering
\includegraphics[width=\linewidth]{images/page_1_A.png}
\caption{Additional qualitative results for room masks and final house layouts. Each row shows four generated sample pairs (i.e. mask and layout) for the same graph presented in the first column. Model was trained on graphs of size 4+ and tested on graphs of size 1-3.}
\label{fig:results_1}
\end{figure*}

\begin{figure*}[t]
\centering
\includegraphics[width=\linewidth]{images/page_2_A.png}
\caption{Continued.}
\label{fig:results_2}
\end{figure*}

\begin{figure*}[t]
\centering
\includegraphics[width=\linewidth]{images/page_1_B.png}
\caption{Results for model trained on graphs of size 1-3 and 7+ and tested on graphs of size 4-6.}
\label{fig:results_3}
\end{figure*}

\begin{figure*}[t]
\centering
\includegraphics[width=\linewidth]{images/page_2_B.png}
\caption{Continued.}
\label{fig:results_4}
\end{figure*}

\begin{figure*}[t]
\centering
\includegraphics[width=\linewidth]{images/page_1_C.png}
\caption{{Results for model trained on graphs of size 1-6 and 10+ and tested on graphs of size 7-9.}}
\label{fig:results_5}
\end{figure*}

\begin{figure*}[t]
\centering
\includegraphics[width=\linewidth]{images/page_2_C.png}
\caption{Continued.}
\label{fig:results_6}
\end{figure*}

\begin{figure*}[t]
\centering
\includegraphics[width=\linewidth]{images/page_1_D.png}
\caption{Results for model trained on graphs of size 1-9 and 13+ and tested on graphs of size 10-12.}
\label{fig:results_7}
\end{figure*}

\begin{figure*}[t]
\centering
\includegraphics[width=\linewidth]{images/page_2_D.png}
\caption{Continued.}
\label{fig:results_8}
\end{figure*}

\begin{figure*}[t]
\centering
\includegraphics[width=\linewidth]{results/page_6.png}
\caption{Results for model trained on graphs of size 1-12 and tested on graphs of size 13+.}
\label{fig:results_9}
\end{figure*}

\begin{figure*}[t]
\centering
\includegraphics[width=\linewidth]{results/page_1.png}
\caption{Continued.}
\label{fig:results_10}
\end{figure*}
